# Supplementary material for: Conformal Lyapunov Optimization: Optimal Resource Allocation under Deterministic Reliability Constraints
Source: arXiv:2503.00486 ancillary file (2025-07-15)
Supplement: Supplementary file 1 [file SupplementalMaterial.pdf]

# Supplemental Material for the manuscript Conformal Lyapunov Optimization: Optimal Resource Allocation under Deterministic Reliability Constraints

## I. LO DERIVATIONS FOR CLO PROTOCOL

We present herein the mathematical derivations to obtain the optimization problem (32) from problem (29) purged of the constraint $(a)$. These derivations are based on the standard LO framework, which firstly envisages to build the Lyapunov function

$$G(t)=\frac{1}{2}\sum_{n=1}^{N}\sum_{k=1}^{K}Q_n^k(t)^2. \quad (1)$$

The Lyapunov function is a measure of the congestion state of the network queues. Specifically, LO is focused on the minimization of the Lyapunov function between consecutive time-slots, namely, the Lyapunov drift (LD), defined as

$$\Delta(t)=\mathbb{E}\{G(t+1)-G(t)|\mathbf{\Gamma}(t)\}, \quad (2)$$

where $\mathbf{\Gamma}(t)=\{Q_n^k(t)\}_{k\in\mathcal{U},n\in\mathcal{N}}$ collects all the transmission queues. Exploiting the following inequality [8]

$$\max(0,(Q-b)+A)^2\leq Q^2+A^2+b^2+2Q(A-b), \quad (3)$$

the LD can be upper-bounded as follows

$$\Delta(t)\leq\sum_{n,k}\xi(n)+\mathbb{E}\left\{Q_n^k(t)\left(\mathbb{1}\{n\in\mathcal{U}\}A^n(t)+\sum_{(l,n)\in\mathcal{E}}R_{l,n}^k(t)\right.\right.$$
$$\left.\left.-\sum_{(n,m)\in\mathcal{E}}R_{n,m}^k(t)-\mathbb{1}\{n\in\mathcal{S}\}I_n^k(t)\right)\middle|\mathbf{\Gamma}(t)\right\}, \quad (4)$$

where, denoting by $\delta_n^+$ and the $\delta_n^-$ the out and the in degree of a node $n$ respectively, we have

$$\xi(n)=1+\frac{\delta_n^{+2}+\delta_n^{-2}}{2}. \quad (5)$$

Specifically, the minimization of (4) pursues the mean-rate stability constraint $(b)$ of (29) [8], without taking into account the objective function (26). Thus, the LD is penalized with the conditional expectation of (26), leading to the Lyapunov Drift Plus Penalty function (LDPP)

$$\Delta_p(t)=\Delta(t)+V\mathbb{E}\{J(t)|\mathbf{\Gamma}(t)\}, \quad (6)$$

where the penalty parameter $V$ is used to explore the trade-off between the objective function (27) and the queue backlogs. Including the penalty in (4), we end up with the following objective function

$$\Delta_p(t)\leq D-\sum_{n\in\mathcal{N},k\in\mathcal{U}}\mathbb{E}\left\{Q_n^k(t)\left(\sum_{(n,m)\in\mathcal{E}}R_{n,m}^k(t)+\mathbb{1}\{n\in\mathcal{S}\}I_n^k(t)\right.\right.$$
$$\left.\left.-A^n(t)\mathbb{1}\{n\in\mathcal{U}\}-\sum_{(l,n)\in\mathcal{E}}\min(R_{l,n}^k(t),Q_l^k(t))\right)\middle|\mathbf{\Gamma}(t)\right\}$$
$$+V\mathbb{E}\left\{\sum_{s\in\mathcal{S},k\in\mathcal{U}}I_s^k(t)F_s^k(t)+V\eta\sum_{k\in\mathcal{U},(n,m)\in\mathcal{E}}R_{n,m}^k(t)E_{n,m}(t)\middle|\mathbf{\Gamma}(t)\right\}, \quad (7)$$

where $D$ is a constant term, given by

$$D=NK+K\sum_{n=1}^{N}\frac{\delta_n^{+2}+\delta_n^{-2}}{2}. \quad (8)$$

According to stochastic optimization we remove the expectations. Then, neglecting the constant terms with respect to the optimization variables and re-arranging the summations, we end up with the instantaneous bound in (32).

## II. DERIVATIONS FOR THE LYAPUNOV BASED OPTIMIZATION PROBLEM

The resource allocation problem based on the classical Lyapunov Optimization framework reads as

$$\begin{aligned}
\underset{\mathbf{\Phi}(t)}{\text{minimize}}\quad & \lim_{T\to\infty}\frac{1}{T}\sum_{t=1}^{T}\mathbb{E}\{J(t)\}\\
\text{subject to}\quad & (a)\ \lim_{f\to\infty}\frac{1}{F}\sum_{f=0}^{F-1}\mathbb{E}\left\{\overline{L_f^k}\right\}\leq r^k,\forall k,\\
& (b)\ Q_n^k(t)\text{ are mean-rate stable }\ \forall k,n,\\
& (c)\ P_n(t)\leq P_n^{\max}\qquad \forall n,t,\\
& (d)\ \sum_{k=1}^{K}I_s^k(t)\leq I_s^{\max}\qquad\forall s,t,\\
& (e)\ \sum_{k=1}^{K}R_{n,m}^k(t)\leq R_{n,m}^{\max}\qquad\forall(n,m)\in\mathcal{E},t
\end{aligned} \quad (9)$$

Constraint $(a)$ is controlled introducing the following virtual queue [8]

$$Z_{f+1}^k=\max(0,Z_f^k+\beta^k(\overline{L_f^k}-r^k)), \quad (10)$$

where $\beta^k$ represents a step-size parameter, used to control the convergence speed of the algorithm, and $\overline{L_f^k}$ is the average loss accrued within the time frame $f$. Specifically, designing a control policy ensuring the mean-rate stability of the queue (10), we also ensure the satisfaction of the long-term constraint defined in (38). To this aim we firstly build the Lyapunov Function

$$G(t,f) = \frac{1}{2}\sum_{n=1}^{N}\sum_{k=1}^{K} Q_n^k(t) + \sum_{k=1}^{K} Z^k(f)^2. \tag{11}$$

Proceeding similarly to the CLO case, exploiting the Lyapunov Drift theorem [8] and the same bound reported in (7), we end up with the following instaneous optimization problem

$$\begin{aligned}\min_{\mathbf{\Phi}(t)}\ & VJ(t) + \sum_{k=1}^{K} Z^k(f)\overline{L_f^k} - \sum_{(n,m)\in\mathcal{E},k\in\mathcal{U}} U_{n,m}^k(t)R_{n,m}^k(t)\\ & -\sum_{n\in\mathcal{N},k\in\mathcal{U}} \mathbb{1}\{n\in\mathcal{S}\}Q_n^k(t)I_n^k(t)\\ \text{s.t.}\ & \text{(9c)-(9e)}.\end{aligned} \tag{12}$$

Note that, while the frame loss $\overline{L_f^k}$ can be used to control the virtual queue evolution, it is not directly related to the control actions, i.e., the decision node selections $\mathbf{I}(t)$ and the threshold values $\mathbf{\Theta}(t)$. Thus, proceeding similarly to [29], we approximate $\overline{L_f^k}$ with a surrogate function, obtained by evaluating the average loss in a portion of the test data

$$\overline{L_f^k} \approx \sum_{s\in\mathcal{S}} I_s^k(t)\tilde{L}_s(\theta^k(t)), \tag{13}$$

where the terms $L_s(\theta^k(t))$ can be modeled through a set of look-up tables, one for each server $s$, storing the average FNR for different values of the hyperparameter $\theta^k$. The overall resource allocation strategy is reported in Algorithm 1.

**Algorithm 1:** Lyapunov Optimization with average reliability constraints.

**Input:** Graph $\mathcal{G} = (\mathcal{N},\mathcal{E})$; time frame duration $S$; and step-sizes $\beta^k$
**Initialize** $\{Z_0^k\}_{k\in\mathcal{U}}$ and $\{Q_n^k(0)\}_{k\in\mathcal{U},n\in\mathcal{N}}$.
**for** $f = 0\dots$ **do**
  set $\{N_f^k = 0\}_{k=1}^K$ and $\{\overline{L}_f^k = 0\}_{k=1}^K$
  **for** $t = fS+1, fS+2, \dots, (f+1)S$ **do**
    solve problem (12), obtaining $\{I_s^{k*}(t), R_{n,m}^{k*}(t), P_{n,m}^*(t), \theta^{k*}(t)\}_{s\in\mathcal{S},(n,m)\in\mathcal{E},k\in\mathcal{U}}$
    **for** $s\in\mathcal{S}$ **do**
      **for** $k\in\mathcal{U}$ **do**
        **if** $I_s^{k*}(t) = 1$ **then**
          get the DU $\tau^k(T_s^k(t))$ at the head of queue $Q_s^k(t)$
          produce a decision $\mathcal{C}_s(\tau^k(T_s^k(t)),\theta(f))$
          evaluate loss $L_t^k = L_s(\tau^k(T_s^k(t)),\theta_f^k)$
          update the average loss $\overline{L}_f^k = \frac{N_f^k}{N_f^k+1}\overline{L}_f^k + \frac{L_t^k}{N_f^k+1}$
          update the number of decisions $N_f^k = N_f^k + 1$
        **end if**
      **end for**
    **end for**
    update the physical queues $\{\{Q_n^k(t+1)\}_{n=1}^N\}_{k=1}^K$ via (20)
  **end for**
  update the virtual queues $\{Z_{f+1}^k\}_{k=1}^K$ using (10),
**end for**
